# Supplementary material for: Kondo effect in binuclear metal-organic complexes with weakly interacting spins
Source: arXiv:1409.6221 source file (2014-09-22)
Supplement: Supplementary file 1 [file Supplementary_Information.pdf]

# Supplementary Information: Kondo effect in binuclear metal-organic complexes with weakly interacting spins

Lei Zhang,[†,‡] Alexei Bagrets,[*,†] Dimitra Xenioti,[¶,†] Richard Korytár,[†] Michael Schackert,[‡] Toshio Miyamachi,[‡,§] Frank Schramm,[†] Olaf Fuhr,[†] Rajadurai Chandrasekar,[‖] Mébarek Alouani,[¶] Mario Ruben,[*,†,¶] Wulf Wulfhekel,[*,‡,†] and Ferdinand Evers[*,⊥,†]

*Institute of Nanotechnology, Karlsruhe Institute of Technology (KIT), Germany, Physikalisches Institut, Karlsruhe Institute of Technology (KIT), Germany, Institut de Physique et Chimie des Matériaux de Strasbourg (IPCMS), Strasbourg, France, Institute of Solid State Physics, University of Tokyo, Japan, School of Chemistry, University of Hyderabad, India, and Institut für Theorie der Kondensierten Materie, Karlsruhe Institute of Technology (KIT), Germany*

E-mail: Alexej.Bagrets@kit.edu; Mario.Ruben@kit.edu; Wulf.Wulfhekel@kit.edu; Ferdinand.Evers@kit.edu

September 22, 2014

[*]To whom correspondence should be addressed
[†]Institute of Nanotechnology, Karlsruhe Institute of Technology (KIT), Germany
[‡]Physikalisches Institut, Karlsruhe Institute of Technology (KIT), Germany
[¶]Institut de Physique et Chimie des Matériaux de Strasbourg (IPCMS), Strasbourg, France
[§]Institute of Solid State Physics, University of Tokyo, Japan
[‖]School of Chemistry, University of Hyderabad, India
[⊥]Institut für Theorie der Kondensierten Materie, Karlsruhe Institute of Technology (KIT), Germany

# I. Electronic structure calculations of free-standing metal-organic complexes

We have employed quantum chemistry packages TURBOMOLE[2] and FHI-aims[1] to analyze electronic structure and magnetic properties of free-standing and adsorbed metal-organic complexes. In particular, in our simulations we have considered free-standing complexes depicted in Suppl. Fig. S1. These are: (a) (Ni(hexafluoroacetylacetonate)$_2$)$_2$bipyrimidine = $Ni_2$ complex, whose atomic structure has been relaxed following data obtained by the single-crystal X-ray diffraction (see Sec. IV.C of SI); (b) "distorted" free-standing $Ni_2$ complex in two slightly different atomic conformations (see also Suppl. Fig. 4), where atomic structures were originated from the relaxation procedure in the presence of Cu(001) surface (see section II.A of SI for further details); and (c) Ni(hexafluoroacetylacetonate)$_2$ = Ni(hfacac)$_2$ moiety. If not stated otherwise, calculations were performed using density functional theory (DFT) within a generalized gradient approximation (GGA) and PBE exchange-correlation functional.[3] In the case of FHI-aims package, a "tier1" basis set composed of numerical atom-centered orbitals has been used. In the case of TURBOMOLE, a basis set of comparable quality, namely, contracted Gaussian-type basis of split-valence quality with polarization functions (def-SVP)[4] has been employed. Furthermore, corresponding Coulomb-fitting basis sets have been used within the resolution of identity approximation.[5]

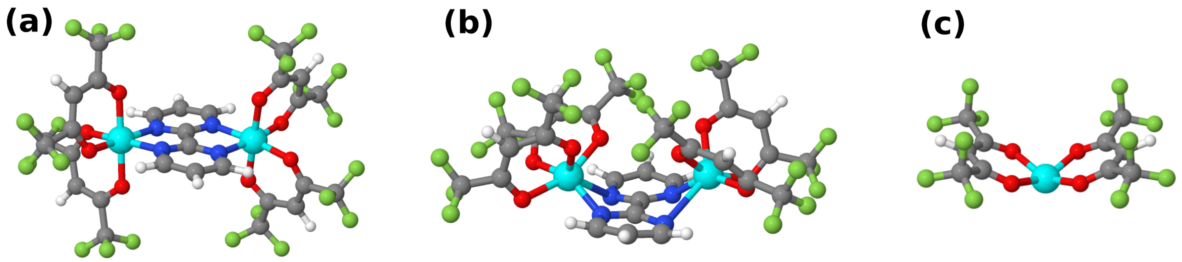


Suppl. Fig. 1: Schematics of atomic structures of metal-organic complexes: (a) free-standing (Ni(hexafluoroacetylacetonate)$_2$)$_2$bipyrimidine = $Ni_2$ complex with Ni(II) ions found in distorted octahedral environment (hydrogen is shown in white; carbon: gray; oxygen: red; nitrogen: dark blue; fluorine: green; and nickel: cyan); (b) $Ni_2$ complex relaxed in the presence of Cu(001) surface (see also Suppl. Fig. 4) with Ni(II) ions found in distorted trigonal prismatic coordination; (c) Ni(hexafluoroacetylacetonate)$_2$ = Ni(hfacac)$_2$ moiety.

Based on the [Ar]3d$^8$ electron configuration of $Ni^{2+}$ ion we anticipate spin-polarized solutions with local magnetic moments of $2\mu_B$ residing primary on Ni centers. These magnetic moments can furthermore be coupled ferro (F)- or antiferromagnetically (AF) for structures (a) and (b) depicted in Suppl. Fig. 1. We have therefore performed "constrained" DFT calculations. Namely, we first prepare an initial guess for the electron density, which is (usually) a superposition of spin-polarized atomic densities, reflecting the presence of two unpaired electrons in the $d$-shell of $Ni^{2+}$ ion. Further, Kohn-Sham (KS) equations have been solved iteratively assuming the number of unpaired electrons in the system to be constrained to 4 (case of F coupled spins) or to zero (case of AF coupled spins). In a similar way, an initial guess for the electron density corresponding to a zero magnetic moment at $Ni^{2+}$ ion can be constructed. In this case, iterative solutions of the KS equations have been converged to an excited state, describing the closed $d$-shell of $Ni^{2+}$ ion, thus breaking Hund's coupling. In the case of $Ni_2$ complexes [structures (a) and (b) in Suppl. Fig. 1], relative energies of magnetic configurations are summarized in Table I (see text of the paper). In the case of Ni(hfacac)$_2$ moiety [structure (c) in Suppl. Fig. 1], we have found the DFT ground state with two unpaired electrons, while the closed shell (excited) state was higher in energy by 0.07 eV.

# II. Electronic structure calculations of molecular complexes on Cu(001) surface

## A. Adsorption geometries

Representative examples of molecular structures adsorbed on Cu(001) surface used in our simulations are shown in Suppl. Figs. 2a, 3a,b and 4. The copper surface has been modeled by finite-size fcc(001)-type atomic clusters, which comprise atoms arranged in few (three or two) atomic layers. Typical clusters contain either 180 (Suppl. Figs. 2a), 121 (Suppl. Fig. S3a), or 107 (Suppl. Fig. S4) Cu atoms, respectively. DFT implemented in the FHI-aims package[1] has been employed to optimize atomic structures of molecules. The calculations have been performed within the

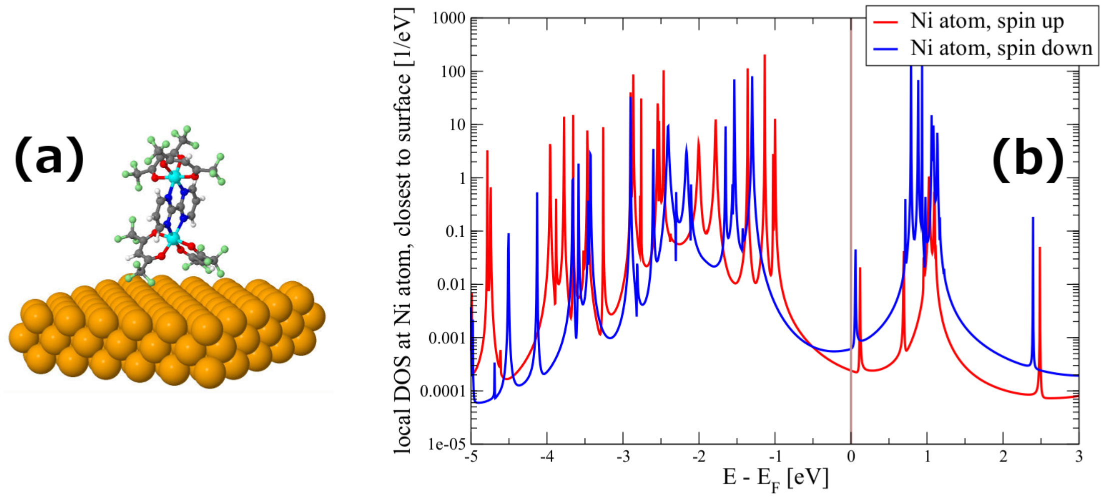


Suppl. Fig. 2: (a) A free-standing-like $Ni_2$ complex bound to a Cu(001) surface via van der Waals forces. In simulations, Cu surface is represented by an fcc-cluster composed of 180 atoms. (b) Spectral function at Ni atom nearest to the surface. A ferromagnetic coupling of $S = 1$ spins residing at $Ni^{2+}$ ions is assumed.

PBE exchange-correlation functional[3] and the "tier1" basis set of numerical atom-centered orbitals. Van der Waals (vdW) contribution to the ground state energy has been accounted for within Tkatchenko-Scheffler model,[6] which relies on the interatomic dispersion coefficients derived from electron density. The atoms of the molecules and few Cu atoms of the surface layer, which are placed in the nearest vicinity of the molecules, have been relaxed. Relaxation steps have been carried out until the residual forces acting on atoms have reached values below 0.01 eV/Å.

In the case of free-standing $Ni_2$ complex relaxed on a surface (see Suppl. Fig. 2a) we have found the F-Cu distances to be about $\sim 3$ Å, suggesting vdW bonding (physisorption) to the surface. This results in a weak hybridization of molecular orbitals with the electronic states of the substrate and, therefore, in extremely narrow resonances, $\sim 10$ meV, seen in the spectral function $A(E)$ projected on a Ni atom (Suppl. Fig. 2b).

In contrast, a Ni(hfacac)$_2$ moiety is strongly bound to a Cu surface (Suppl. Fig. 3a,b), so that a significant hybridization of the molecular orbitals is present in the spectral function (Suppl. Fig. 3c). In this case, a chemical bond is realized through Ni atom placed in the "hollow" site. Furthermore, our calculations indicate (see Fig. 4b of the paper) that the energetically most favorable adsorption

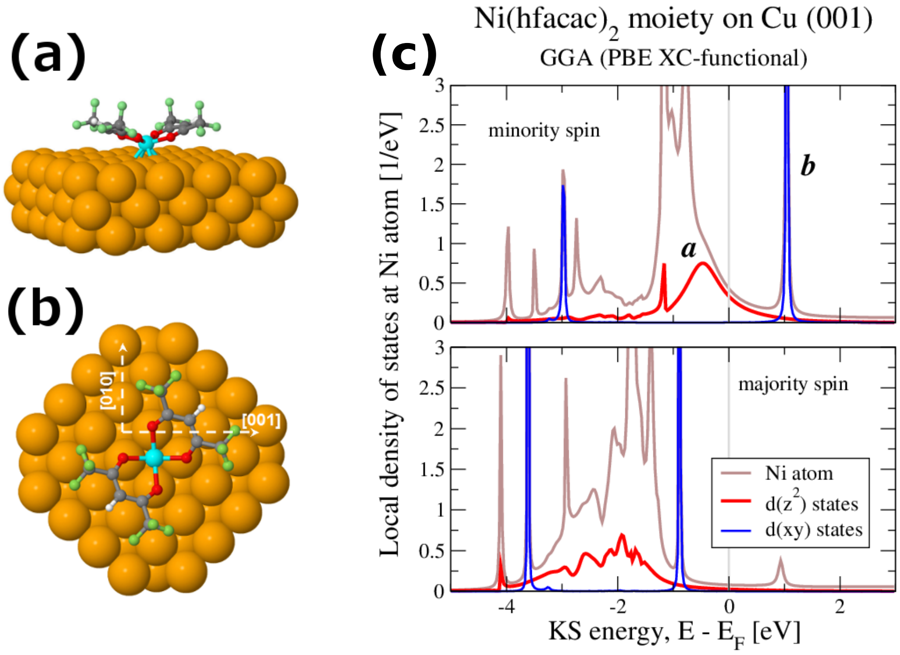


Suppl. Fig. 3: (a) Side view and (b) top view of the Ni(hfacac)$_2$ moiety bound to a Cu(001) surface, with Ni atom placed in the "hollow" position. Energetically favorable conformation, according to the DFT calculation, corresponds to a mirror plane of Ni(hfacac)$_2$ being rotated by 45° with respect to the crystallographic axises of the fcc (001) surface. (c) Spectral function $A(E)$ at Ni atom, computed within the generalized gradient approximation (GGA, PBE exchange-correlation functional[3]). Red and blue lines highlight contributions to $A(E)$ associated with Ni $d_{z^2}$-type and $d_{xy}$-type orbitals, marked $a$ and $b$ respectively (cf. Fig. 5 of the paper, where GGA+$U$ corrected method[7,8] is employed, leading to the minority $a$ orbital being shifted above the Fermi level).

configuration is realized when symmetry planes of the Ni(hfacac)$_2$ moiety are rotated by 45° with respect to [001] and [010] crystallographic directions of the fcc (001) surface (see Suppl. Fig. 3b): thus oxygen atoms are placed "on-top" of Cu atoms. This observation correlates with the experimental STM images of adsorbed Ni$_2$-$\alpha$ spices ("equal-sign" objects in Suppl. Figs. 5d,e), which are misaligned relative to basic crystallographic directions of the surface plane.

Also in the case of "distorted" molecular confirmation of Ni$_2$ complex (see Suppl. Fig. 4) our simulations indicate that a chemical bond is established between the molecule and the Cu surface. This bond is presumably realized via the delocalized $\pi$-orbitals of the bipyrimidine (bpym) unit, which are overlapping with the electron density extending from the surface. The bond has also an ionic character due to fractional charge transfer $\sim 0.5e$ to the LUMOs (see subsection IV.D of the

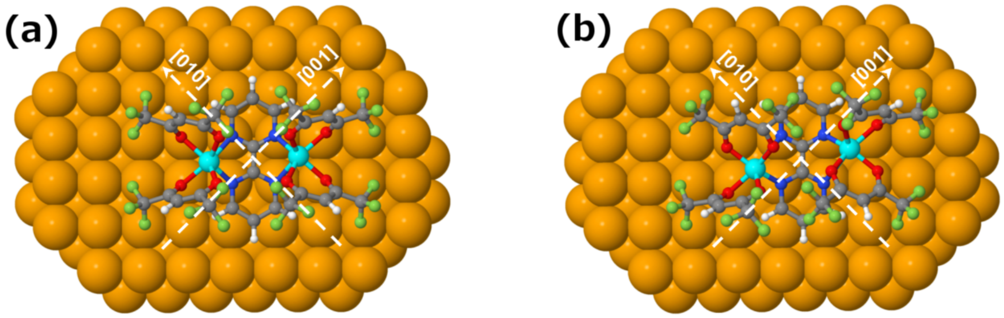


Suppl. Fig. 4: Schematics of two "distorted" molecular conformations of $Ni_2$ complex adsorbed on a Cu(001) surface via the bpym unit: (a) almost symmetric $C_{2v}$-type structure with two mirror planes of the molecular complex rotated by 45° relative to fcc [001] and [010] directions; (b) energetically more stable structure with a broken local symmetry.

paper). A binding geometry is characterized by a relatively short N-Cu bond length of 0.205 Å, where N atoms are placed almost "on top" of the corresponding Cu atoms of the surface. More specifically, in our analysis (see e.g. data presented in Table I of the paper) we have considered two slightly different conformations of "distorted" $Ni_2$ complex. A molecular conformation shown in Suppl. Fig. 4a has been obtained within the preliminary DFT relaxation procedure: the atomic structure of the complex has an approximate $C_{2v}$ symmetry, consistent with the underlying fcc(001) surface, and atomic forces have been converged up to 0.1 eV/Å. We note also that such a molecular conformation reveals simulated STM images with a "cross-like" structure, whose orientation on the surface is consistent with experimentally observed $Ni_2$-$\beta$ species (see Fig. 5f). Further relaxation steps (accounting for the energy gain of around $\sim 0.25$ eV) break local symmetry of the molecular complex resulting in the molecular conformation shown in Suppl. Fig. 4b.

## B. Embedded approach and spectral function

Spectral functions of molecular complexes adsorbed on a Cu(001) surface have been calculated within the non-equilibrium Green's function (NEGF) formalism merged with DFT. An approach, which we follow here, has been used successfully in our previous works and is implemented in a homemade simulation code AITRANSS,[9–11] interfaced to the FHI-aims[1] and TURBOMOLE[2] packages. In brief, we consider a metal-organic complex bound to an atomic Cu cluster as an "extended

molecule", which is coupled to an infinite "reservoir" of electrons. The Cu clusters used in these simulations are typically smaller as compared to the ones the that have been chosen for the relaxation of molecular structures on surfaces. These smaller clusters are limited to the two outermost atomic layers of the Cu(001) surface and contain, respectively, 84, 57 and 82 Cu atoms in the cases of the systems illustrated in Suppl. Fig. 2 [free-standing $Ni_2$ complex on Cu(001)], Suppl. Fig. 3 [Ni(hfacac)$_2$ moiety on Cu(001)] and Suppl. Fig. 4 [distorted $Ni_2$ complex on Cu(001)]. The corresponding "extended molecules" comprise 2978, 1883 and 2920 electrons, respectively.

After a self-consistent set of Kohn-Sham (KS) orbitals is found for the "extended molecule", its interaction with the infinite reservoir of electrons has been accounted for within the Green's function formalism. Namely, the KS Hamiltonian is supplemented by the parameter-dependent local self-energy, $\Sigma^{\rm surface}(\mathbf{x},\mathbf{x}') = [\lambda - i\eta]\,\delta(\mathbf{x}-\mathbf{x}')$, which is ascribed to the "surface-1" atomic layer of the simulation clusters. For the chosen value $\eta$ of the level broadening ($\eta = 2.7$ eV in present calculations), the contribution $\lambda$ to the real part of the self-energy is obtained by imposing the charge neutrality condition within the "extended molecule". Its Green's function is further projected out on the basis functions associated with selected atoms (e.g. Ni ions) thus allowing to compute partial (local) density of states (see Suppl. Figs. 2b, 3b and figures in the paper).

## C. Simulation of STM images

According to Tersoff and Hamann,[12] STM images can be approximated by the space-resolved local density of states. In our numerical simulations, we have used two computational methods, which follow this approach. First, we have employed embedded technique and the Green's function formalism linked to the quantum-chemical "cluster"-type calculations, as implemented in the AITRANSS package. Details of the implementation are given in our previous work.[10] Specifically, we have plotted a space-resolved spectral function (in close vicinity of the molecular complexes), which has been integrated over an energy window of 0.1 eV around the Fermi level. We have confronted our results with those obtained using the pseudopotential VASP code.[13] In the latter simulations, we have employed a quasi two-dimensional (2D) supercell set-up, with the 2D Bril-

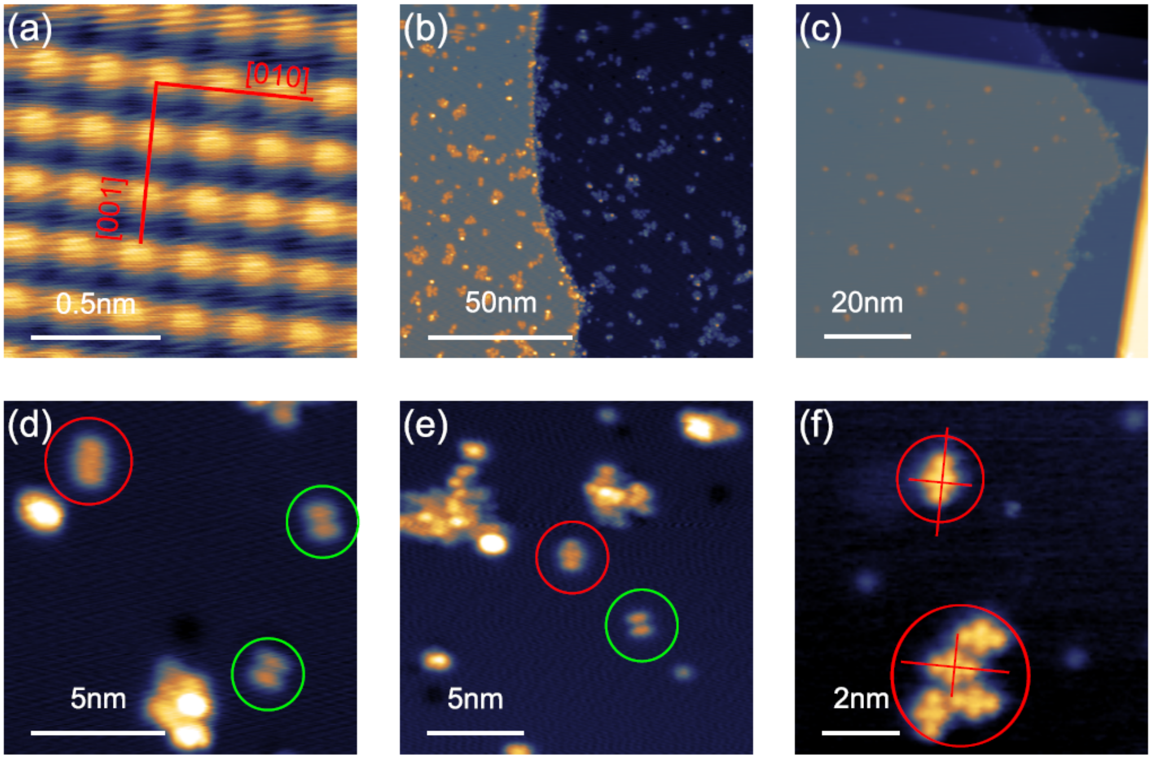


Suppl. Fig. 5: A series of STM images characterizing adsorption of $Ni_2$ complexes on a Cu(001) surface. (a) Cu(100) surface with atomic resolution. (b) $Ni_2$/Cu(100) sample. $Ni_2$ was evaporated at 105°C within 20 seconds. (c) $Ni_2$/Cu(100) sample. $Ni_2$ was evaporated at 100°C within 10 seconds. (d),(e) $Ni_2$/Cu(100) sample. $Ni_2$ was evaporated when a substrate was at room temperature. Two kinds of single objects could be recognized: (1) a "plus-sign" type in red circle ($Ni_2$-$\beta$), (2) an "equal-sign" type in green circle ($Ni_2$-$\alpha$). (f) $Ni_2$/Cu(100) sample. $Ni_2$ was evaporated when a substrate was pre-cooled in the STM chamber. Only the "plus-sign" object ($Ni_2$-$\beta$) can be found on the Cu surface. The symmetry axes of the "plus-sign" object ($Ni_2$-$\beta$) always follow the [010] and [001] direction of the substrate.

louin zone mapped by $16 \times 16$ **k**-points, and a plane waves basis set with 500 eV energy cut-off. Both computational methods provide us with STM images, qualitatively consistent with each other (cf. Figs. 4 and 6 of the paper).

# III. Calculation of the electron-phonon coupling constants

We have employed quantum chemistry package TURBOMOLE[2] to estimate the electron-phonon coupling constants of the "Kondo-active" molecular orbitals to vibrational modes of a $Ni_2$ complex.

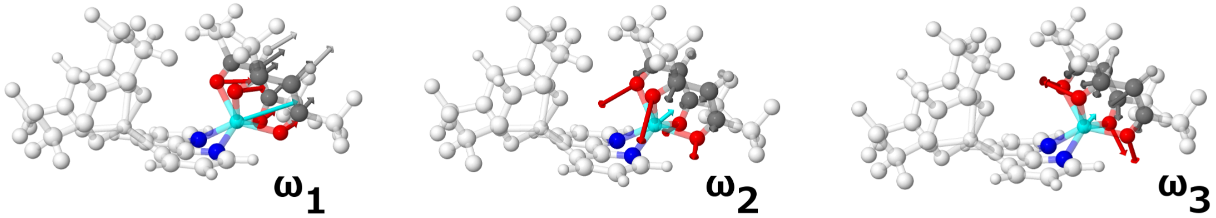


Suppl. Fig. 6: Schematic representation of the low-energy vibrational eigenmodes ($\omega_1 = 25.1$ meV, $\omega_2 = 32.6$ meV, $\omega_3 = 33.4$ meV, displacements are scaled by $\times 10$) of distorted $Ni_2$ complex, which are localized within the "active" subspace limited to one Ni ion and surrounding 14 atoms, shown in color (see text of the paper and SI for further details).

The analysis of molecular vibrations was performed in the harmonic approximation by solving the eigenvalue problem for a mass-weighted Hessian matrix, which was evaluated semi-analytically as outlined in Ref. 14. The matrix elements $M^{\mu}_{mn}$ of the (second-quantized) electron-phonon interaction of the form $\sum_{\mu} M^{\mu}_{nm}(b^{\dagger}_{\mu} + b_{\mu}) d^{\dagger}_{n} d_{m}$, involving vibrational modes $\mu$ and a pair of Kohn-Sham (KS) molecular orbitals $m$ and $n$, can be computed based on the first-order derivatives of the KS operator $H^{\mathrm{KS}}$ with respect to nuclear displacements $\delta\mathbf{R}_a$:

$$M^{\mu}_{nm} = \sum_{\mathbf{R}_a}^{\text{atoms}} \sqrt{\frac{\hbar}{2M(\mathbf{R}_a)\omega_{\mu}}} \sum_{i=x,y,z} u^{i}_{\mu}(\mathbf{R}_a) \left\langle n \left| \frac{\partial H^{\mathrm{KS}}}{\partial(\delta R^{i}_{a})} \right| m \right\rangle .$$

Here $\mathbf{u}_{\mu}(\mathbf{R}_a)$ are normal modes (normalized eigenvectors of the mass-weighted Hessian matrix), $\omega_{\mu}$ the corresponding frequencies, and the KS Hamiltonian $H^{\mathrm{KS}}$ comprises electrostatic potential of ions and single-particle contributions due to kinetic energy, Hartree- and exchange-correlation terms (see Ref. 15 for further details). In a nutshell, the matrix element $M^{\mu}_{nm}$ is the energy cost for a shift of the atoms from their equilibrium positions by the elementary oscillator lengths, $\sqrt{\hbar/M(\mathbf{R}_a)\omega_{\mu}}$, into the direction of the normal mode at hand.

We have argued in the paper (Sections IVC,D) that for a particular example of "distorted" $Ni_2$ complex, each of the two Ni ions develops the Kondo effect independently, so that our analysis of the electron-phonon coupling may be limited to the "active" subspace (Suppl. Fig. 6). This subspace comprises a Ni ion and its surrounding of 14 atoms (2 nitrogens, 4 oxygens, 6 carbons

and 2 hydrogen atoms), which are "embedded" into an otherwise rigid organic cage. Specifically, we have computed the diagonal matrix elements $\lambda^{\mu} = M^{\mu}_{KK}$, where $K$ refers to the molecular orbital involved in the formation of Kondo resonance (see Fig. 9b of the paper). Within the energy window below 50 meV, only three low-energy eigenmodes ($\omega_1 = 25.1$ meV, $\omega_2 = 32.6$ meV, $\omega_3 = 33.4$ meV) were found to have non-zero electron phonon-coupling constants: they are illustrated in Suppl. Fig. 6. Such a selection can be rationalized as follows: a "Kondo-active" molecular orbital has a contribution arising from atomic $3d$ orbital of the Ni ion, whose on-site energy is controlled by the splitting of the $d$ shell. This splitting is modulated provided a motion of Ni and O atoms substantially modifies the local environment of the Ni ion, which is indeed the case for the three selected eigenmodes shown in Suppl. Fig. 6. In the case of other vibrations, the change of the on-site energy is a second order effect with respect to the eigenmodes' displacements.

# IV. Synthesis of molecular complexes, crystal structures and magnetic measurements data

## A. General remarks

The commercially available initial materials, 2,2'-bipyrimidine (bpym) and Me(hfacac)$_2$ (Me= Ni, Mn, Zn), as well as all solvents were used as received without further purification from various suppliers such as Sigma-Aldrich, VWR and ABCR. Reported preparation procedures to synthesize the binuclear complexes were partially adapted from Refs. 16,17 and are summarized in Suppl. Fig. 7.

X-ray crystallographic data collection[18] for the $[(Ni(hfacac)_2)_2(bpym)]^0$ and $[(Mn(hfacac)_2)_2$-(bpym)$]^0$ complexes were performed with a STOE IPDS II diffractometer and with graphite-monochromated Mo-K$\alpha$ radiation at 200 K for $Ni_2$ and 180 K for $Mn_2$, respectively. The structure was solved by direct methods (SHELX-97).[19] Refinement was carried out with anisotropic temperature factors for all non-hydrogen atoms by means of full-matrix least squares techniques against Fo2 (SHELXTL97-2, Refs. 19,20).

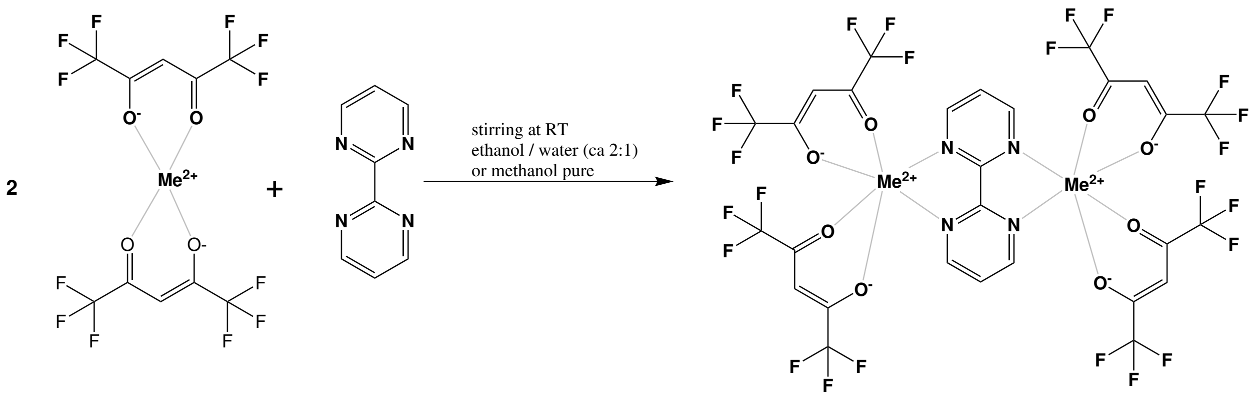


Suppl. Fig. 7: Preparation pathway to synthesize the $[(Me(hfacac)_2)_2(bpym)]^0$ complexes with Me = $Ni^{2+}$, $Mn^{2+}$ and $Zn^{2+}$.

Temperature dependent static susceptibilities of $[(Ni(hfacac)_2)_2(bpym)]^0$ and $[(Mn(hfacac)_2)_2$-(bpym)$]^0$ were recorded with an MPMS-5S (Quantum Design) SQUID magnetometer over a temperature range of 1.9–300 K in a homogeneous 0.1 T external magnetic field. Gelatin capsules were used as sample containers. The diamagnetic corrections of the molar magnetic susceptibilities were applied using well-known Pascal's constants.[21]

## B. $[(Ni(hfacac)_2)_2(bpym)]^0$: synthesis

89 mg(0.5 mmol) of 2,2'-bipyrimidine (bpym) and 473 mg (1 mmol) $Ni(hfacac)_2$ were dissolved in 30 ml of a 3:1 mixture of ethanol/water and stirred over night at room temperature; after that a pale green precipitate was formed. Reduction of the solvent in vacuum to about 10 ml volume increased amount of the solid. The residual solvent was filtered off and the solid was washed twice with a mixture of ethanol/water (1:1). The solid was dried in vacuum (10 mbar) and then sublimated twice in vacuum ( $8 \cdot 10^{-3}$ mbar, 175–185°C). The sublimated solid yielded 195 mg (35%) of a pure compound.

Suppl. Table 1: Selected bond lengths and bond angles of $[(Ni(hfacac)_2)_2(bpym)]^0$ obtained from single crystal X-ray diffraction data.

| Bond | distance, Å | Bond angle | degrees |
|---|---|---|---|
| Ni(1)-O(4) | 2.000(3) | O(4)-Ni(1)-O(2) | 91.84(14) |
| Ni(1)-O(2) | 2.025(3) | O(4)-Ni(1)-O(1) | 86.12(13) |
| Ni(1)-O(1) | 2.034(3) | O(2)-Ni(1)-O(1) | 90.57(12) |
| Ni(1)-O(3) | 2.038(3) | O(4)-Ni(1)-O(3) | 90.00(13) |
| Ni(1)-N(1) | 2.086(3) | O(2)-Ni(1)-O(3) | 89.65(12) |
| Ni(1)-N(3) | 2.112(3) | O(1)-Ni(1)-O(3) | 176.12(12) |
| Ni(2)-O(5) | 2.028(3) | O(4)-Ni(1)-N(1) | 172.41(13) |
| Ni(2)-O(6) | 2.029(3) | O(2)-Ni(1)-N(1) | 94.98(13) |
| Ni(2)-O(7) | 2.031(3) | O(1)-Ni(1)-N(1) | 90.49(12) |
| Ni(2)-O(8) | 2.031(3) | O(3)-Ni(1)-N(1) | 93.35(12) |
| Ni(2)-N(4) | 2.112(3) | O(4)-Ni(1)-N(3) | 93.82(14) |
| Ni(2)-N(2) | 2.113(3) | O(2)-Ni(1)-N(3) | 174.26(12) |
| | | O(1)-Ni(1)-N(3) | 88.94(12) |
| | | O(3)-Ni(1)-N(3) | 91.23(12) |
| | | N(1)-Ni(1)-N(3) | 79.31(13) |
| | | O(4)-Ni(1)-O(2) | 91.84(14) |

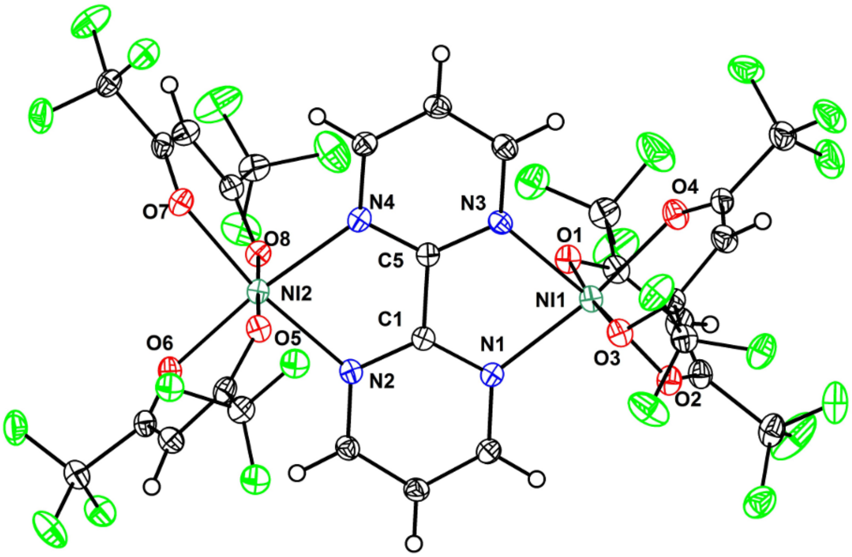


Suppl. Fig. 8: Ortep plot of the molecular structure of the $[(Ni(hfacac)_2)_2(bpym)]^0$ complex obtained by single crystal X-ray diffraction. Ellipsoids are depicted with 20% probability, C (black), O (red), N (blue), F (light green), Ni (dark green), H (black circles).

## C. $[(Ni(hfacac)_2)_2(bpym)]^0$: data from single crystal X-ray diffraction

Crystallization of the $[(Ni(hfacac)_2)_2(bpym)]^0$ complex occurred upon slow evaporation of a dichloromethane solution of the reaction product and the obtained crystals were suitable for single crystal X-ray diffraction. Selected bond distances and angles are summarized in Suppl. Table 1. Data analysis reveals that the two Ni atoms are coordinated by the oxygen atoms of two hexafluoroacetylacetonato ligands and two nitrogen atoms of the bridging bipyrimidine ligand (see Suppl. Fig. 8). Together these ligands construct a distorted octahedral coordination sphere around the Ni. Bond distances between Ni and oxygen atoms (2.00–2.04 Å) are shorter than between Ni and nitrogen atoms (2.09–2.11 Å). Bond angles within the pentanedionato-ligands (O-Ni-O) are close to ideal 90°. The N-Ni-N angle is considerably smaller (79.38°). The distance between the two Ni atoms is about 5.60 Å. The trifluoromethyl groups are significantly disordered, which is expressed by large vibrational ellipses in Suppl. Fig. 8.

## D. $[(Ni(hfacac)_2)_2(bpym)]^0$: magnetic measurements

Magnetic susceptibility data and field dependence measurements were carried out on powder samples of the sublimated compound. Effective magnetic moment, molar magnetic susceptibility and its reciprocal were determined between 6 and 300 K (see Suppl. Figs. 9 and 10). At 300 K an effective magnetic moment of 4.22 $\mu_B$ was detected, which compares well with reported values between 3.0 $\mu_B$ (at ca. 110 K)[16] and 4.49 $\mu_B$.[17] Spin only value corresponds to $\mu_{eff} = 4.90\ \mu_B$, but this neglects slight anisotropic effects. Intramolecular antiferromagnetic interaction between the metal ions within the dimer at low temperatures can be derived from susceptibility data as well as from the reciprocal susceptibility. A maximum value of the molar magnetic susceptibility has been found at 17 K, which is in very good agreement with a reported value.[16] Linear fit (Curie-Weiss law) of the reciprocal molar susceptibility data above $T > 50$ K results in a Curie constant $\theta = -20.89$ K. Below 50 K the $1/\chi_{mol}$ curve deviates from linear behavior to exhibit an increase which corresponds to the described antiferromagnetic coupling.

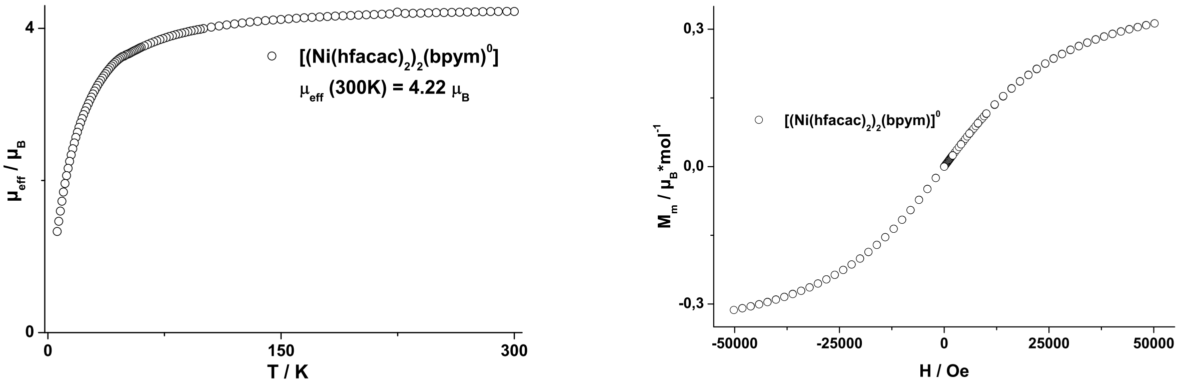


Suppl. Fig. 9: Magnetic measurements data of $[(Ni(hfacac)_2)_2(bpym)]^0$. Left: effective magnetic moment ($\mu_{eff}$ in $\mu_B$) at 0.1 T field. Right: field dependence of the molar magnetic moment at $T = 2$ K.

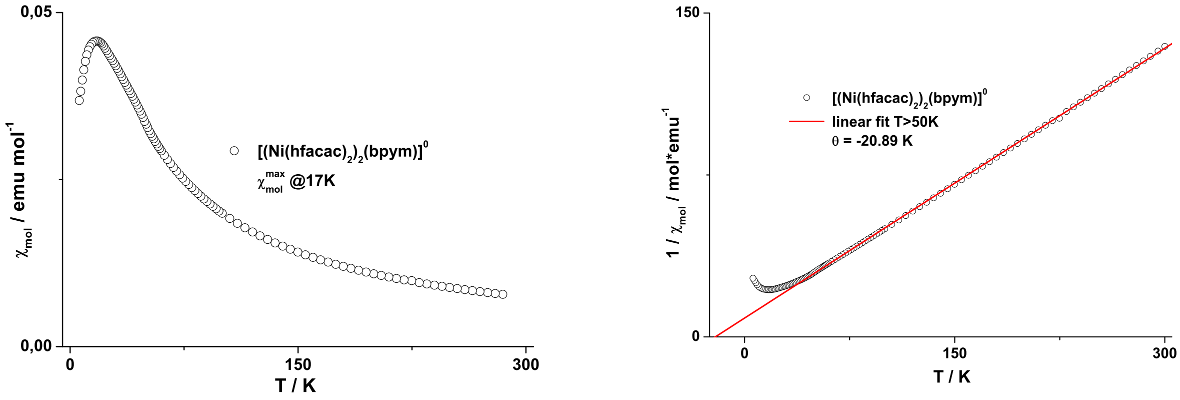


Suppl. Fig. 10: Magnetic measurements data of $[(Ni(hfacac)_2)_2(bpym)]^0$. Left: molar magnetic susceptibility at 0.1 T field. Right: reciprocal molar susceptibility measured at 0.1 T. Black circles depict the experimental values, the red line is the linear fit.

## E. $[(Mn(hfacac)_2)_2(bpym)]^0$: synthesis

*Pathway A*. 15.2 mg(0.1 mmol) of 2,2'-bipyrimidine (bpym) and 126.3 mg (0.25 mmol) $Mn(hfacac)_2$-*$2H_2O$ were dissolved in 20 ml methanol and stirred over night at room temperature. The solvent was removed and the yellow solid was washed twice with a mixture of ethanol/water (1:1). The solid was dried in vacuum (10 mbar) and then sublimated in vacuum ($2 \cdot 10^{-2}$ mbar, 150–160°C). The sublimated solid yielded 78 mg (53%) of pure compound.

*Pathway B*. 0.79 g (0.5mmol) of 2,2'-bipyrimidine and 0.469g (1mmol) of $Mn(hfacac)_2$*$2H_2O$ were dissolved in 125 ml of a mixture of $CH_2Cl_2$/hexane (1:1) and the whole solution was allowed to evaporate slowly at room temperature. After 7 days yellow color crystal dinuclear Mn(II) crystalline complex was formed. The crystals were hand-picked to give yield of ca. 150 mg.

## F. $[(Mn(hfacac)_2)_2(bpym)]^0$: data from single crystal X-ray diffraction

The crystals obtained from a synthetic procedure (*Pathway B*) were suitable for single crystal X-ray diffraction measurement, which results the molecular structure. Selected bond distances and bond angles are shown in Suppl. Table 2. Data analysis reveals that the two manganese ions are coordinated by two hexafluoroacetylacetonato ligands each, and — at one side — by the bipyrimidine bridging ligand (Suppl. Fig. 11). Surprisingly, the metal ion is placed in a distorted trigonal-prismatic coordination environment of two N atoms (bpym) and four O atoms (hfacac).

The bonds lengths between Mn and oxygen atoms are shorter (2.13–2.19 Å) than the ones between Mn and nitrogen atoms (2.29–2.33 Å). But these values are considerably larger than the ones of the $[(Ni(hfacac)_2)_2(bpym)]^0$ (see Section IV.C). This points to a significantly weaker ligand field strength in the case of $[(Mn(hfacac)_2)_2(bpym)]^0$. Also the O-Mn-O bond angles of the acetylacetonato ligands are much less and are close to the ideal 90 degrees value (81–83°). Furthermore, the N-Mn-N angles (71°) are as well smaller compared with N-Ni-N angle, which in total manifests a distinct distortion of the coordination sphere. This can be correlated to the larger atomic radius of the Mn ions in comparison to the Ni ions.

Suppl. Table 2: Selected bond lengths and bond angles of $[(Mn(hfacac)_2)_2(bpym)]^0$ obtained from single crystal X-ray diffraction data.

| Bond | distance, Å | Bond angle | degrees | Bond angle | degrees |
|---|---|---|---|---|---|
| Mn(1)-O(3) | 2.131(4) | O(3)-Mn(1)-O(1) | 86.40(15) | O(6)-Mn(2)-O(8) | 147.17(17) |
| Mn(1)-O(1) | 2.141(3) | O(3)-Mn(1)-O(4) | 82.21(13) | O(6)-Mn(2)-O(7) | 90.52(14) |
| Mn(1)-O(4) | 2.148(3) | O(1)-Mn(1)-O(4) | 131.16(13) | O(8)-Mn(2)-O(7) | 81.86(14) |
| Mn(1)-O(2) | 2.187(3) | O(3)-Mn(1)-O(2) | 151.01(14) | O(6)-Mn(2)-O(5) | 81.48(14) |
| Mn(1)-N(1) | 2.294(4) | O(1)-Mn(1)-O(2) | 80.97(13) | O(8)-Mn(2)-O(5) | 85.32(15) |
| Mn(1)-N(2)#1 | 2.334(3) | O(4)-Mn(1)-O(2) | 86.65(12) | O(7)-Mn(2)-O(5) | 142.39(16) |
| Mn(2)-O(6) | 2.138(4) | O(3)-Mn(1)-N(1) | 118.04(14) | O(6)-Mn(2)-N(3) | 124.20(14) |
| Mn(2)-O(8) | 2.142(4) | O(1)-Mn(1)-N(1) | 138.10(13) | O(8)-Mn(2)-N(3) | 83.15(14) |
| Mn(2)-O(7) | 2.142(3) | O(4)-Mn(1)-N(1) | 87.86(12) | O(7)-Mn(2)-N(3) | 130.53(15) |
| Mn(2)-O(5) | 2.146(4) | O(2)-Mn(1)-N(1) | 88.03(13) | O(5)-Mn(2)-N(3) | 82.26(15) |
| Mn(2)-N(3) | 2.318(4) | O(3)-Mn(1)-N(2)#1 | 83.11(13) | O(6)-Mn(2)-N(4)#2 | 81.41(15) |
| Mn(2)-N(4)#2 | 2.319(4) | O(1)-Mn(1)-N(2)#1 | 80.07(12) | O(8)-Mn(2)-N(4)#2 | 128.56(16) |
| | | O(4)-Mn(1)-N(2)#1 | 144.14(12) | O(7)-Mn(2)-N(4)#2 | 82.68(14) |
| | | O(2)-Mn(1)-N(2)#1 | 119.76(13) | O(5)-Mn(2)-N(4)#2 | 131.44(15) |
| | | N(1)-Mn(1)-N(2)#1 | 70.72(12) | N(3)-Mn(2)-N(4)#2 | 70.92(13) |

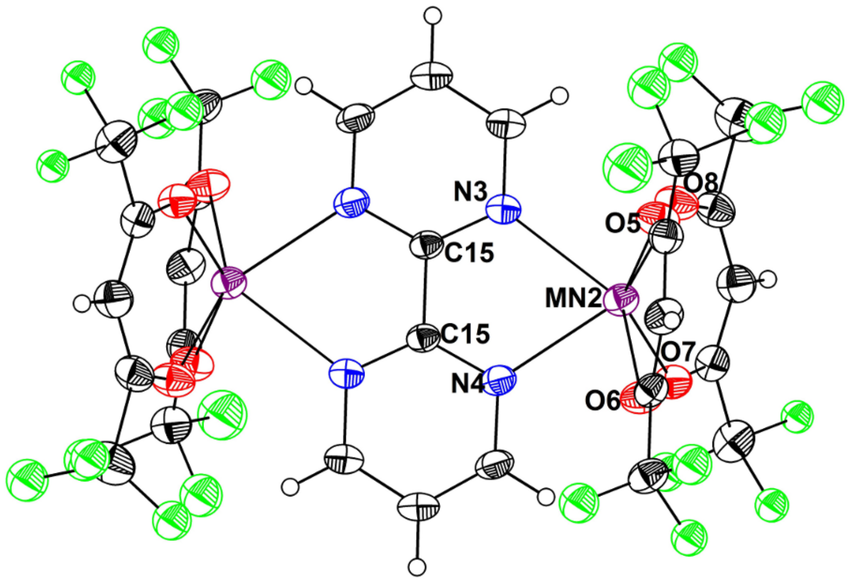


Suppl. Fig. 11: Ortep plot of the molecular structure of the $[(Mn(hfacac)_2)_2(bpym)]^0$ complex obtained by single crystal X-ray diffraction. Ellipsoids are depicted with 20% probability, C (black), O (red), N (blue), F (light green), Mn (violet), H (black circles).

The intermetallic distance between Mn-Mn of 6.16 Å is also clearly longer than in the Ni analogue. Apparently, the trigonal prismatic coordination environment causes such an increase in distance and, as a consequence, the reduction of magnetic interaction between the metal ions within the dimer. Also, the trifluoromethyl groups are largely disordered, which causes the undefined refinement of the fluorine atoms. The position of each F atom was therefore calculated on three (adjacent) positions within the molecular structure.

## G. $[(Mn(hfacac)_2)_2(bpym)]^0$: magnetic measurements

Magnetic susceptibility data and field dependence measurements were carried out on powder samples of the sublimated compound. Effective magnetic moment, molar magnetic susceptibility and its reciprocal were determined between 2 and 300 K (see Suppl. Figs. 12 and 13). At 300 K an effective magnetic moment of 8.50 $\mu_B$ was detected, which compares well with the spin only value of $\mu_{eff} = 8.37\ \mu_B$. In early reports by Brewer & Sinn,[16] Mn(II)-bipyrimidyl-Mn(II) complexes exhibited the same behavior. Relatively weak intramolecular antiferromagnetic interaction between the Mn(II) ions within the dimer at low temperatures can be derived from susceptibility data, as well as from the reciprocal susceptibility. A maximum value of the molar magnetic susceptibility has been found at 3.95 K. Linear fit of the reciprocal molar susceptibility data above $T > 12$ K results in a Curie-constant $\theta = -4.11$ K. Below 12 K, the $1/\chi_{mol}$-curve deviates from linear behavior and exhibits an increase, which corresponds to the mentioned antiferromagnetic coupling.

## H. $[(Zn(hfacac)_2)_2(bpym)]^0$: synthesis and magnetic measurements

89 mg(0.5 mmol) of 2,2'-bipyrimidine (bpym) was dissolved in 20 ml of a 3:1 mixture of ethanol/water and 545 mg (1 mmol) $Zn(hfacac)_2*2H_2O$ were dissolved in 15 ml of a 1:1 mixture of ethanol/water. The Zn solution was added slowly to the bpym solution and the mixture was stirred over night at room temperature to form a little amount of white precipitate. Removal of the solvents in vacuum to about 10 ml yielded more solid material. The residual solvent was filtered off and the solid was washed twice with 10 ml of a mixture of ethanol/water (1:1). The solid was

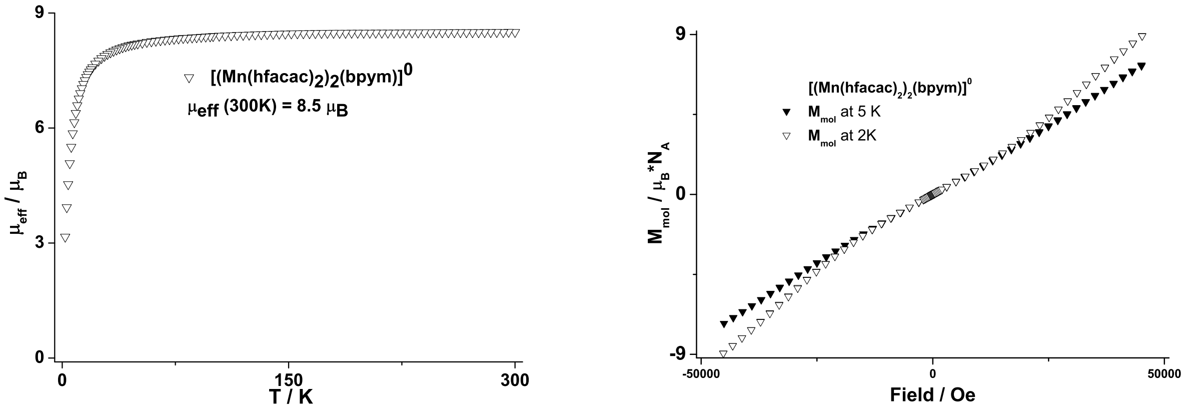


Suppl. Fig. 12: Magnetic measurements data of $[(Mn(hfacac)_2)_2(bpym)]^0$. Left: effective magnetic moment ($\mu_{eff}$ in $\mu_B$) at 0.1 T field. Right: field dependence of the molar magnetic moment at $T = 2$ K and $T = 5$ K.

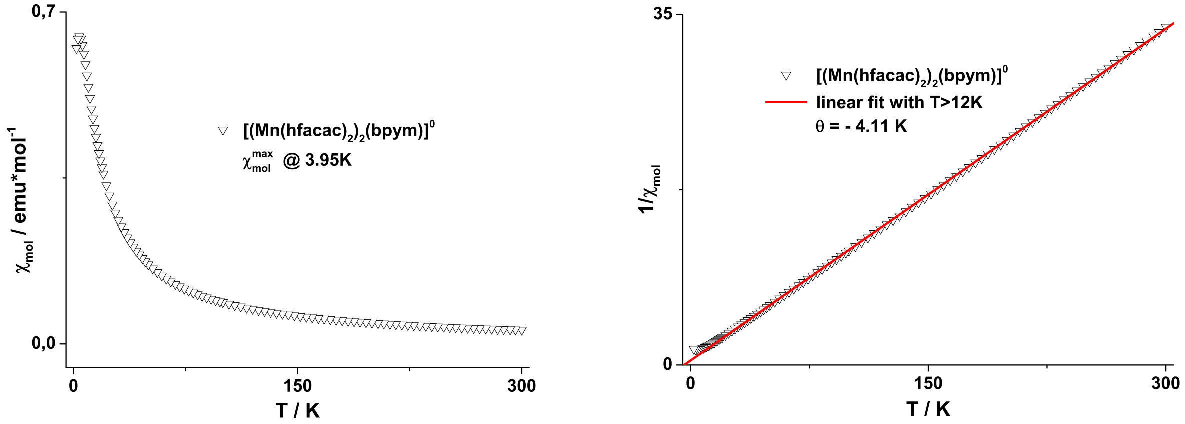


Suppl. Fig. 13: Magnetic measurements data of $[(Mn(hfacac)_2)_2(bpym)]^0$. Left: molar magnetic susceptibility at 0.1 T field. Right: reciprocal molar susceptibility measured at 0.1 T. Black triangles depict the experimental values, the red line is the linear fit.

dried in vacuum (10 mbar) and weighed out to yield 488 mg (87%) of white solid. 108 mg of the compound was sublimated in vacuum ($1.4 \cdot 10^{-2}$ mbar, 135–145°C). The sublimated solid yielded 62 mg (57%) of pure compound.

The molar magnetic susceptibility was determined at 300 K and 0.1 T. The resulting value, $\chi_{\mathrm{mol}} = -1.34 \cdot 10^{-3}$ emu/mol, describes a purely diamagnetic material.

## References


(1) V. Blum, R. Gehrke, F. Hanke, P. Havu, V. Havu, X. Ren, K. Reuter, and M. Scheffler, Comp. Phys. Comm. **180**, 2175-2196 (2009).

(2) R. Ahlrichs, *et al.* TURBOMOLE 6.6 (development version), program package for *ab initio* electronic structure calculations, Turbomole GmbH (2014).

(3) J. P. Perdew, K. Burke, and M. Ernzerhof, Phys. Rev. Lett. **77**, 3865 (1996).

(4) A. Schäfer, H. Horn, and R. Ahlrichs, J. Chem. Phys. **97**, 2571 (1992)

(5) K. Eichkorn, O. Treutler, H.Öhm, M. Häser, and R. Ahlrichs, Chem. Phys. Lett. **242**, 652 (1995).

(6) A. Tkatchenko and M. Scheffler, Phys. Rev. Lett. **102**, 073005 (2009).

(7) V. I. Anisimov, F. Aryasetiawan, and A. I. Lichtenstein, J. Phys.: Condens. Matt. **9** 767 (1997).

(8) S. Kümmel and L. Kronik, Rev. Mod. Phys. **80**, 3–60 (2008).

(9) A. Arnold, F. Weigend, and F. Evers, J. Chem. Phys. **126**, 174101 (2007).

(10) J. Wilhelm, M. Walz, M. Stendel, A. Bagrets, and F. Evers, Phys. Chem. Chem. Phys. **15**, 6684 (2013).

(11) A. Bagrets, J. Chem. Theory Comput. **9**, 2801 (2013).

(12) J. Tersoff and D. R. Hamann, Phys. Rev. B **31**, 805-813 (1985).

(13) G. Kresse and J. Furthmüller, Phys. Rev. B **54**, 11169 (1996).

(14) P. Deglmann, K. May, F. Furche, and R. Ahlrichs, Chem. Phys. Lett. **384**, 103 (2004); P. Deglmann, F. Furche, and R. Ahlrichs, Chem. Phys. Lett. **362**, 511 (2004); P. Deglmann and F. Furche, J. Chem. Phys. **117**, 9535 (2002).

(15) M. Bürkle, J. K. Viljas, T. J. Hellmuth, E. Scheer, F. Weigend, G. Schön, and F. Pauly, Phys. Status Solidi B **250**, 2468 (2013).

(16) G. Brewer and E. Sinn, Inorg. Chem. **24**, 4580 (1985); ibid. **23**, 2532 (1985)

(17) M. Barquín, M. J. G. Garmendia, and V. Bellido, Trans. Met. Chem. **24**, 546 (1999).

(18) A listing of data collection and refinement procedures as well as positional coordinates of all atoms (CIF files) were deposited at the Cambridge Crystallographic Data Centre under CCDC-1023858 for $[(Ni(hfacac)_2)_2(bpym)]^0$, and CCDC-1023859 for $[(Mn(hfacac)_2)_2(bpym)]^0$, respectively, which contain the supplementary crystallographic data excluding structure factors. These data can be obtained free of charge via `www.ccdc.cam.ac.uk/conts/retrieving.html` (or from the Cambridge Crystallographic Data Centre, 12, Union Road, Cambridge CB2 1EZ, UK; Fax: (+44) 1223-336-033; or `deposit@ccdc.cam.ac.uk`).

(19) G. M. Sheldrick, *A short history of SHELX.* Acta Cryst. A **64**, 112 (2008).

(20) G. M. Sheldrick, *SHELXTL97-2*, University of Göttingen, Germany (1997).

(21) G. A. Bain and J. F. Berry, J. Chem. Educ. **85**, 532 (2008).
